# Supplementary material for: ShadowMaskFormer: Mask Augmented Patch Embeddings for Shadow Removal
Source: arXiv:2404.18433 source file (2025-03-22)
Supplement: Supplementary file 1 [file 7-appendix.tex]

In this supplementary materials, we include: more details on the search space in Section~\ref{sec:app_search_space}, more details on the proposed method in Section~\ref{sec:app_approach}; \textcolor{black}{visualizations of the obtained architectures in Figure~\ref{fig:architectures}}; and a further analysis on the Huawei Atlas 200 DK in Section~\ref{sec:atlas_supp}.

\section{Search Space and Encoding Continued \label{sec:app_search_space}}

Designing a search space that is expressive but also tractable has been a key element to the success of NAS algorithms \cite{nasnet2018,mnasnet}. The generality of the chosen search space has a major influence on the kinds of architectures that are even possible. While the tractability ensures good models can be identified by a principled algorithm within a reasonable time frame. In this work, we follow the encoder-decoder architectural framework, which has been proven successful for the task of semantic segmentation \cite{chen2018encoder}. 

The encoder aims to extract higher-level contextual information at multiple scales via gradually downsampled feature maps, which is very similar to the backbone\footnote{all layers prior to the last linear classification layer.} part of a CNN for object classification. The decoder aims to aggregate the extracted multi-scale features (from the encoder) to derive lower-level spatial information for locating objects. In this work, we leverage the BiSeNet \cite{yu2018bisenet} heads as the decoder, and focus on designing the encoder. A pictorial illustration is provided in Fig.~1 in the main paper. 

\begin{table}[!hbt]
\centering
\caption{\textbf{Architecture Schema:} The searched encoder architecture is based on ResNet \cite{resnet}, including the input image scale ($r$), depth ($d_i$), and the width ($m_i$, $\vec{e}_i$). The detailed setting is presented using $\begin{bmatrix}{k} \times k\mbox{, \#Ch}\end{bmatrix}$, where $k$ denotes the convolution filter size, \#Ch denotes the number of output channels, and $\begin{bmatrix} \cdot \end{bmatrix}$ indicates residual connection. $^{\dagger}$indicates the locations for outputting features. The ResNet-50 architecture is also provided for reference.\label{tab:search-space}}
\resizebox{.6\textwidth}{!}{%
\begin{tabular}{@{\hspace{2mm}}c|c|c|c@{\hspace{2mm}}}
\toprule
\multicolumn{1}{l|}{} & \multicolumn{1}{c|}{output scale} & \multicolumn{1}{c|}{ResNet-50 \cite{resnet}} & \multicolumn{1}{c}{\ourmethod{}} \\ \midrule
\multirow{3}{*}{Stem} & \multirow{3}{*}{$\frac{r}{2}$ $\times$ $\frac{r}{2}$} & \multirow{3}{*}{7 $\times$ 7, 64, stride 2} & 3 $\times$ 3, 32, stride 2 \\
 &  &  & $\begin{bmatrix} \mbox{3} \times \mbox{3, 32}\end{bmatrix}$ $\times$ $d_0$ \\
 &  &  & 3 $\times$ 3, 64 $\times$ $m_0$ \\ \midrule
\multirow{5}{*}{Stage 1} & \multirow{5}{*}{$\frac{r}{4}$ $\times$ $\frac{r}{4}$} & \multicolumn{2}{c}{3 $\times$ 3 max pool, stride 2} \\ \cmidrule(l){3-4} 
 &  & $\begin{bmatrix} \mbox{1} \times \mbox{1, 64}\\ \mbox{3} \times \mbox{3, 64}\\ \mbox{1} \times \mbox{1, 256}\end{bmatrix}$ $\times$ 3 & $\begin{bmatrix} \mbox{1} \times \mbox{1, 64} \times \vec{e}_1\\ \mbox{3} \times \mbox{3, 64} \times \vec{e}_1\\ \mbox{1} \times \mbox{1, 256} \times m_1\end{bmatrix}$ $\times$ $d_1$ \\ \midrule
\multirow{1}{*}{Stage 2} & \multirow{1}{*}{$\frac{r}{8}$ $\times$ $\frac{r}{8}$} & $\begin{bmatrix} \mbox{1} \times \mbox{1, 128}\\ \mbox{3} \times \mbox{3, 128}\\ \mbox{1} \times \mbox{1, 512}\end{bmatrix}$ $\times$ 3 & $\begin{bmatrix} \mbox{1} \times \mbox{1, 128} \times \vec{e}_2\\ \mbox{3} \times \mbox{3, 128} \times \vec{e}_2\\ \mbox{1} \times \mbox{1, 512} \times m_2\end{bmatrix}$ $\times$ $d_2$ \\ \midrule
\multirow{1}{*}{Stage 3$^{\dagger}$} & \multirow{1}{*}{$\frac{r}{16}$ $\times$ $\frac{r}{16}$} & $\begin{bmatrix} \mbox{1} \times \mbox{1, 256}\\ \mbox{3} \times \mbox{3, 256}\\ \mbox{1} \times \mbox{1, 1024}\end{bmatrix}$ $\times$ 3 & $\begin{bmatrix} \mbox{1} \times \mbox{1, 256} \times \vec{e}_3\\ \mbox{3} \times \mbox{3, 256} \times \vec{e}_3\\ \mbox{1} \times \mbox{1, 1024} \times m_3\end{bmatrix}$ $\times$ $d_3$ \\ \midrule
\multirow{1}{*}{Stage 4$^{\dagger}$} & \multirow{1}{*}{$\frac{r}{32}$ $\times$ $\frac{r}{32}$} & $\begin{bmatrix} \mbox{1} \times \mbox{1, 512}\\ \mbox{3} \times \mbox{3, 512}\\ \mbox{1} \times \mbox{1, 2048}\end{bmatrix}$ $\times$ 3 & $\begin{bmatrix} \mbox{1} \times \mbox{1, 512} \times \vec{e}_4\\ \mbox{3} \times \mbox{3, 512} \times \vec{e}_4\\ \mbox{1} \times \mbox{1, 2048} \times m_4\end{bmatrix}$ $\times$ $d_4$ \\ \midrule
\multirow{1}{*}{Tail$^{\dagger}$} & \multirow{1}{*}{1 $\times$ 1} & \multicolumn{2}{c}{global average pool} \\
\bottomrule
\end{tabular}%
}
\end{table}

For each stage, we allow the \# of layers to vary from two to four (four to six for stage 3), and apply stride of two to the first layer to half the feature map size (except the first stage where a max pooling with stride 2 is used). Additionally, we allow the output \# of channels ($m_i$) to vary from $0.6\times$ to $1\times$ of the default values. For each layer, we allow the output \# of channels of the first $1\times1$ convolution ($\vec{e}_i$) to vary from $0.8\times$ to $1.4\times$ of the default values. The choices of the feature-outputting locations are implicitly controlled by the depth settings as we always output the features of the last layers from the final two stages and tail. Table~\ref{tab:search-space} summaries our architectural decision space. And example of our encoding is provided in Fig.~\ref{fig:encoding}.

\begin{figure}[!hbt]
    \centering
    \begin{subfigure}{0.6\textwidth}
    \centering
    \includegraphics[width=.98\textwidth{}]{figures/encoding_resnet.pdf}
    \end{subfigure}
\caption{\textbf{Encoding:} An integer-valued string is used to encode searchable architectures comprising a stem and four stages. The leading two digits encode the \# of layers ($d_i$) and the output \# of channels ($m_i$). For stages, the remaining digits encode the intermediate \# of channels ($\vec{e}_i$) for each layer in the stage. Zeros are padded to the stage strings to avoid variable-length representations. See Table~\ref{tab:search-space} for more details. \label{fig:encoding}}
\end{figure}

\section{Proposed method Continued\label{sec:app_approach}}
\vspace{2pt}
\noindent\textbf{-- Initialization:}
Recall that our method is an evolutionary process in which initial solutions are made gradually better as a group. Instead of starting from a completely random set of solutions (i.e., architectures), we follow a customized initialization procedure shown in Algorithm~\ref{algo:init}. It ensures that the extreme solutions (i.e., most and least complex architectures) are always parts of the initial population, in the spirit of enhancing diversity. Empirically, we observe that this initialization method leads to better surrogate modeling performance, which in turn improves the performance of the subsequent evolutionary search for optimal architectures.

\begin{center}
\begin{minipage}{.6\textwidth}
\begin{algorithm}[H]
\SetAlgoLined
\SetKwInOut{Input}{Input}
\SetKwInOut{Output}{Output}
\SetKwFor{For}{for}{do}{end for}
\normalsize
\Input{Population size $N$, hypernetwork $\mathcal{H}$, validation data $\mathcal{D}_{vld}$, archive $\mathcal{A}$.}
    $i$ $\leftarrow$ 0 \textcolor{gray}{// initialize an individual counter}.\\
    $P$, $F_p$ $\leftarrow$ $\emptyset$ \textcolor{gray}{// initialize parent population}.\\
    \While{$i < N$}{
    \uIf{i $==$ 0}{
        \textcolor{gray}{// Set individual to the lower bound of the search space}. \\
        $p$ $\leftarrow$ $lower$ $bound$ \\
      }
      \uElseIf{i $==$ 1}{
        \textcolor{gray}{// Set individual to the upper bound of the search space}. \\
        $p$ $\leftarrow$ $upper$ $bound$ \\
      }
      \Else{
        $p$ $\leftarrow$ randomly sample an individual from the search space. \\
      }
    $F$ $\leftarrow$ $Evaluate$($p$, $\mathcal{H}$, $\mathcal{D}_{vld}$) \hspace{12mm} $\triangleleft$ Algo~2 (main paper)\\
    $P$, $F_p$ $\leftarrow$ $P$ $\cup$ $p$, $F_p$ $\cup$ $F$ \\
}
$\mathcal{A}$ $\leftarrow$ $\mathcal{A}$ $\cup$ ($P$, $F_p$) \\
\textbf{Return} $P$, $F_p$, $\mathcal{A}$ 
\caption{Initialization \label{algo:init}}
\end{algorithm}
\end{minipage}
\end{center}

\vspace{2pt}
\noindent\textbf{-- Segmentation accuracy prediction:}
most selection operators in existing EAs (such as binary tournament selection, non-dominated sorting, etc.) merely require relative relationships among individuals instead of specific fitness values. 
For example, given two candidate solutions A and B, it is sufficient for selection operators to proceed by knowing either $f_A > f_B$ or $f_A < f_B$, while the absolute difference between the fitness of them (i.e., $\lVert f_A-f_B \rVert$) is not required. 
Hence, we argue that ``a low MSE is desirable but not necessary''. 

Considering such a context, our motivation is to design a computationally efficient surrogate model to substitute the time-costly evaluation via the supernet, where the fundamental requirement is that the rank correlation between the predicted values and the actual values should be sufficiently high. 
Therefore, we replace the standard loss of MSE (Eq. (4)) with a ranking-based loss (Eq. (5)) for learning the surrogate model. A pictorial illustration is provided in Figure~\ref{fig:rank_loss_sketch}.

\begin{figure}[ht]
\centering
\includegraphics[width=.8\textwidth{}]{revision_r1/rank_loss_sketch.pdf}
\caption{Considering five pairs of the true (\textbf{\textcolor{green}{green}} circles) and predicted (\textbf{\textcolor{violet}{purple}} triangles) values. An MSE loss aims to minimize the Euclidean distance between the true and predicted values (i.e., left sub-figure). While a ranking-based loss aims to maintain the same ranking between sorting based on the true and predicted values (right sub-figure). For the purpose of differentiating architectures during an EA process, a high-rank correlation is required, while a low MSE is desirable but not required. \label{fig:rank_loss_sketch}}
\end{figure}

\vspace{2pt}
\noindent\textbf{-- Pre-screening:}
Recall that the pre-screening criterion adopted in our method for in-fill selection inherits an inductive bias towards the objective that is (relatively speaking) computationally friendly to (high-fidelity) evaluate, i.e., inference latency. To realize this goal, we formulate the problem as a subset selection problem and solve it using a customized binary genetic algorithm (GA). The modifications introduced to a conventional GA consider the feasibility in solution creation steps (i.e., initialization, crossover, and mutation) to improve the efficiency of the algorithm. The detailed procedures are outlined in Algorithm ~\ref{algo:bGA}.

\begin{center}
\begin{minipage}{.78\textwidth}
\begin{algorithm}[H]
\SetAlgoLined
\SetKwInOut{Input}{Input}
\SetKwInOut{Output}{Output}
\SetKwFor{For}{for}{do}{end for}
\normalsize
\Input{Population size $N$, max. \# of generations $T$,\\total \# of candidate solutions $L$,\\max. \# of solutions to be selected $K$.}
    \textcolor{gray}{// initialization} \\
    $i$ $\leftarrow$ 0, $P$ $\leftarrow$ $\emptyset$\\
    \While{$||P|| < N$}{
        $p$ $\leftarrow$ $zeros$($L$) \\
        $k$ $\leftarrow$ create a random integer less than $K$.\\
        $idx$ $\leftarrow$ create a set of permutation indices of length $L$.\\
        $p\big[idx[:k]\big]$ $\leftarrow$ $1$ \\ 
        $P$ $\leftarrow$ $P$ $\cup$ $p$ \\
    }
    \While{$t < T$}{
        $Q$ $\leftarrow$ $\emptyset$ \\
        \While{$||Q|| < N$}{
            $p_1$, $p_2$ $\leftarrow$ binary tournament selection ($P$)\\
            \textcolor{gray}{// crossover} \\
            $q$ $\leftarrow$ $zeros$($L$) \\
            $idx_{1}$ $\leftarrow$ AND($p_1$, $p_2$) \textcolor{gray}{// find indices where both $p1$ \& $p2$ take value ``1''.}\\
            $q$\big[$idx_{1}$\big] $\leftarrow$ 1 \\ 
            $idx_{2}$ $\leftarrow$ XOR($p_1$, $p_2$) \textcolor{gray}{// find indices where at least one parent takes value ``1''.}\\
            $k$ $\leftarrow$ create a random integer less than $K - ||idx_{1}||$. \\
            $q$\big[$idx_{2}[:k]$\big] $\leftarrow$ 1 \\
            \textcolor{gray}{// mutation} \\
            $q$ $\leftarrow$ randomly flip a ``0'' to ``1'' \\
            $q$ $\leftarrow$ randomly flip a ``1'' to ``0'' \\
        }
        $P$ $\leftarrow$ Survive($P$ $\cup$ $Q$, $N$) \textcolor{gray}{// survive the top-K ranked solutions.}
    }
\textbf{Return} $P$
\caption{Customized Binary GA\label{algo:bGA}}
\end{algorithm}
\end{minipage}
\end{center}

\iffalse
\vspace{2pt}
\noindent\textbf{-- Decision Making:}
The proposed multi-objective algorithm is expected to produce a set of non-dominated solutions trading-off segmentation accuracy and inference speed. In absence of explicit user preferences, we resort to \emph{trade-off}, as an unsupervised metric, to select architectures. Assuming a minimization problem of M objectives, the trade-off of the $i$-th solution is calculated as the average loss per unit average gain among its nearest neighbors $B(i)$ based on the Euclidean distance in the normalized objective space, as follows:

\begin{equation}
\small
\begin{aligned}
% \mbox{Trade-off}(i) = \max_{j=1}^{|B(i)|}\frac{{\rm Avg. Loss}(i,j)}{{\rm Avg. Gain}(i,j)}
\mbox{Trade-off}(i) = \max_{j \in B(i)}\frac{\mathbb{E}\big(Loss(i,j)\big)}{\mathbb{E}\big(Gain(i,j)\big)},
\end{aligned}
\label{def:trade-off}
\normalsize
\end{equation}

\noindent where 
\begin{equation}
\small
\begin{aligned}
\mathbb{E}\big(Loss(i,j)\big) &=& \frac{\sum_{k=1}^M \max\big(0, f_k(j) -
  f_k(i)\big)}{\sum_{k=1}^M \big\{1| f_k(j) >
  f_k(j)\big\}},\\
\mathbb{E}\big(Gain(i,j)\big) &=& \frac{\sum_{k=1}^M \max\big(0, f_k(i) -
  f_k(j)\big)}{\sum_{k=1}^M \big\{1| f_k(i) >
  f_k(j)\big\}}.
\end{aligned}
\normalsize
\end{equation}

For a solution, a higher trade-off value indicates that it causes a larger average loss in some objectives to make a unit average gain in other objectives choose any of its nearest neighbors. Thereby, we select solutions with trade-off values that are significantly larger (e.g., over two standard deviations; from a statistical point of view) than others. 
\fi

\begin{figure}[ht]
    \centering
    \includegraphics[width=0.9\textwidth{}]{figures/architectures.pdf}
    \caption{\textcolor{black}{MoSegNets-\{small, median, large\} architectures from Table II in the main paper. Architectures are arranged in descending inference-speed order from top to bottom. \label{fig:architectures}}}
\end{figure}

\section{Application to Huawei Atlas 200 DK Continued\label{sec:atlas_supp}}
Based on the experimental results shown in Section~VI of the main paper, we observe a weak correlation between inference latency on the Huawei Atlas 200 DK and on GPUs, such as RTX 2080 Ti. Towards facilitating a better understanding on the characteristics of the run-time latency on Huawei Atlas 200 DK, the following experiments have been performed. We sample a large number of 4K architectures uniformly from our search space. For each model, we compute the semantic segmentation accuracy (mIoU) on Cityscapes dataset using the weights inherited from the hypernetwork (Section III-C in the main paper), with an additional 2K iterations of fine-tuning. In the meantime, we also measure \#Params, \#FLOPs and the run-time latency on both Atlas and 2080Ti for each model. Fig.~\ref{fig:atlas_analysis} depicts the experimental results. In general, we observe that the latency on Atlas 200 DK is relatively more correlated with latency on 2080 Ti, as oppose to \#FLOPs, \#Params. And it's surprising that there exists high-performing architectures across all levels of latency (on Atlas 200 DK). 

\begin{figure}[t]
    \centering
    \begin{subfigure}[b]{\textwidth}
    \centering
    \includegraphics[width=\textwidth{}]{figures/visualize_atlas.pdf}
    \end{subfigure}
\caption{Visualization of the trade-off between the inference latency on the Huawei Atlas 200 DK and \{Cityscapes mIoU, RTX 2080 Ti latency, \#FLOPs, \#Params\}, from left to right respectively.\label{fig:atlas_analysis}}
\end{figure}
